# Supplementary material for: Three-Dimensional Venus Cloud Structure Simulated by a General Circulation Model
Source: arXiv:2407.15966 source file (2024-07-22)
Supplement: Supplementary file 1 [file Shao_2023_VenusClouds_R3_SI.pdf]

# Supporting Information for "Three-Dimensional Venus Cloud Structure Simulated by a General Circulation Model"

Wencheng D. Shao[1], Joao Mendonca[1], Longkang Dai[2]

[1]National Space Institute, Technical University of Denmark, Lyngby, Denmark

[2]College of Meteorology and Oceanography, National University of Defense Technology, Changsha, China

## Contents of this file

1. Figures S1 to S8

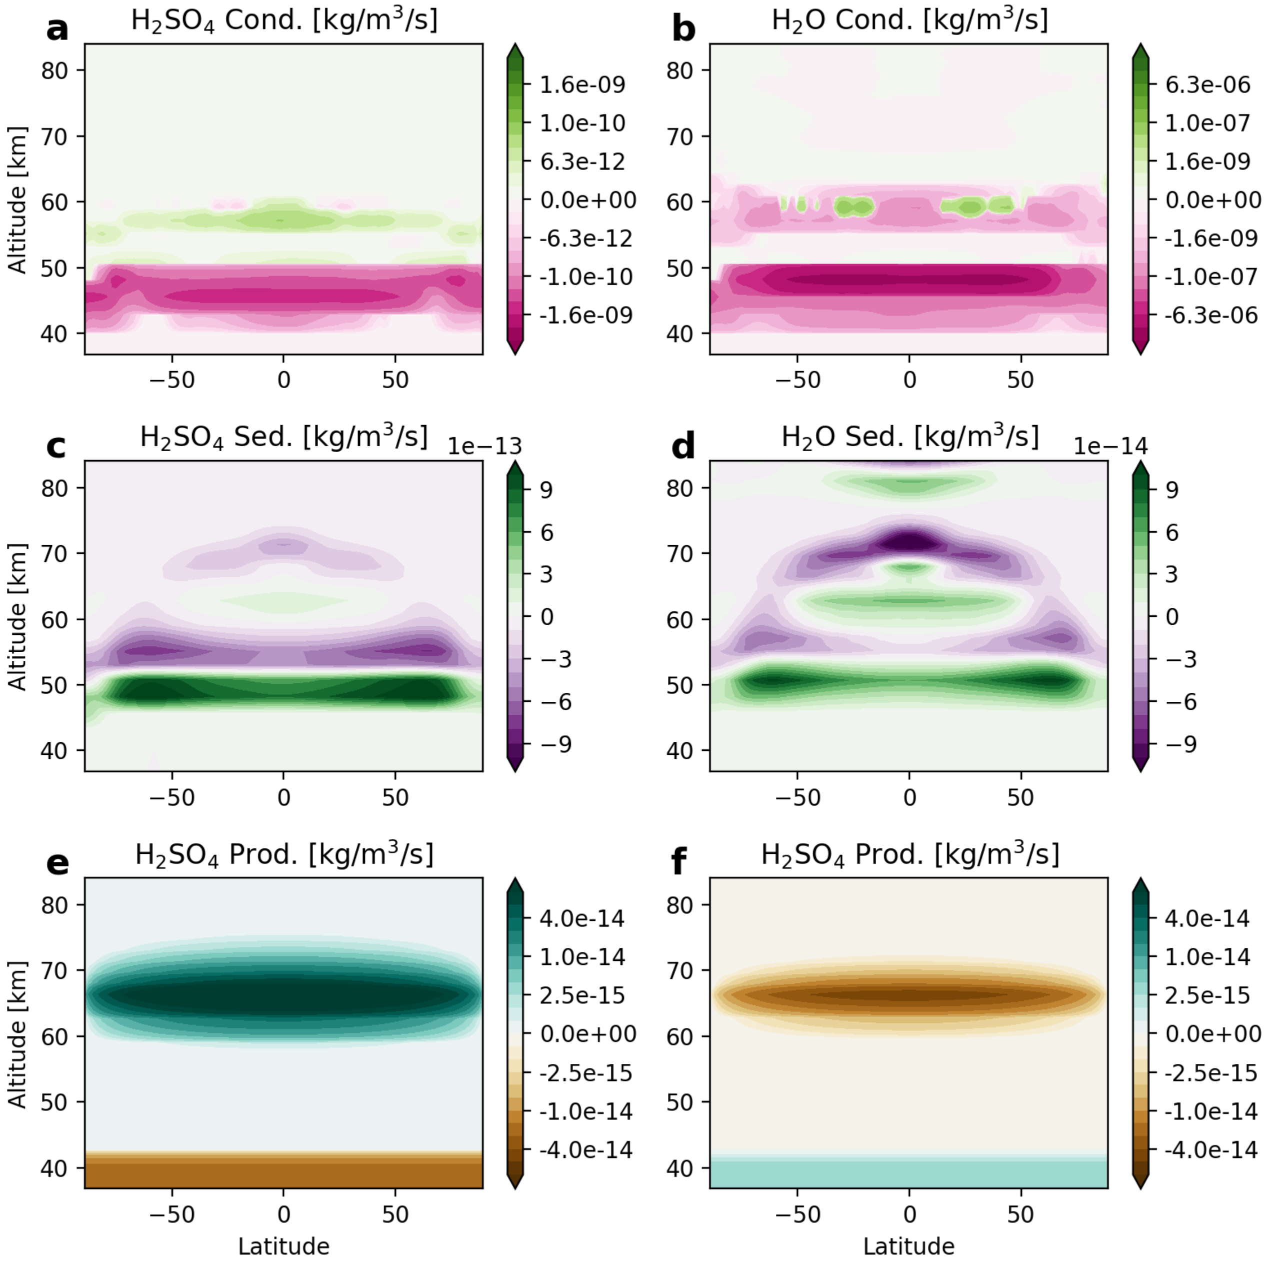


**Figure S1.** Simulated (a) $H_2SO_4$ condensation rate (unit: $kg\,m^{-3}\,s^{-1}$), (b) $H_2O$ condensation rate (unit: $kg\,m^{-3}\,s^{-1}$), (c) $H_2SO_4$ sedimentation rate (units: $kg\,m^{-3}s^{-1}$), (d) $H_2O$ sedimentation rate (units: $kg\,m^{-3}\,s^{-1}$), (e) $H_2SO_4$ vapor production rate (unit: $kg\,m^{-3}\,s^{-1}$) and (f) $H_2O$ vapor production rate (unit: $kg\,m^{-3}\,s^{-1}$) averaged zonally and over the last Venus day.

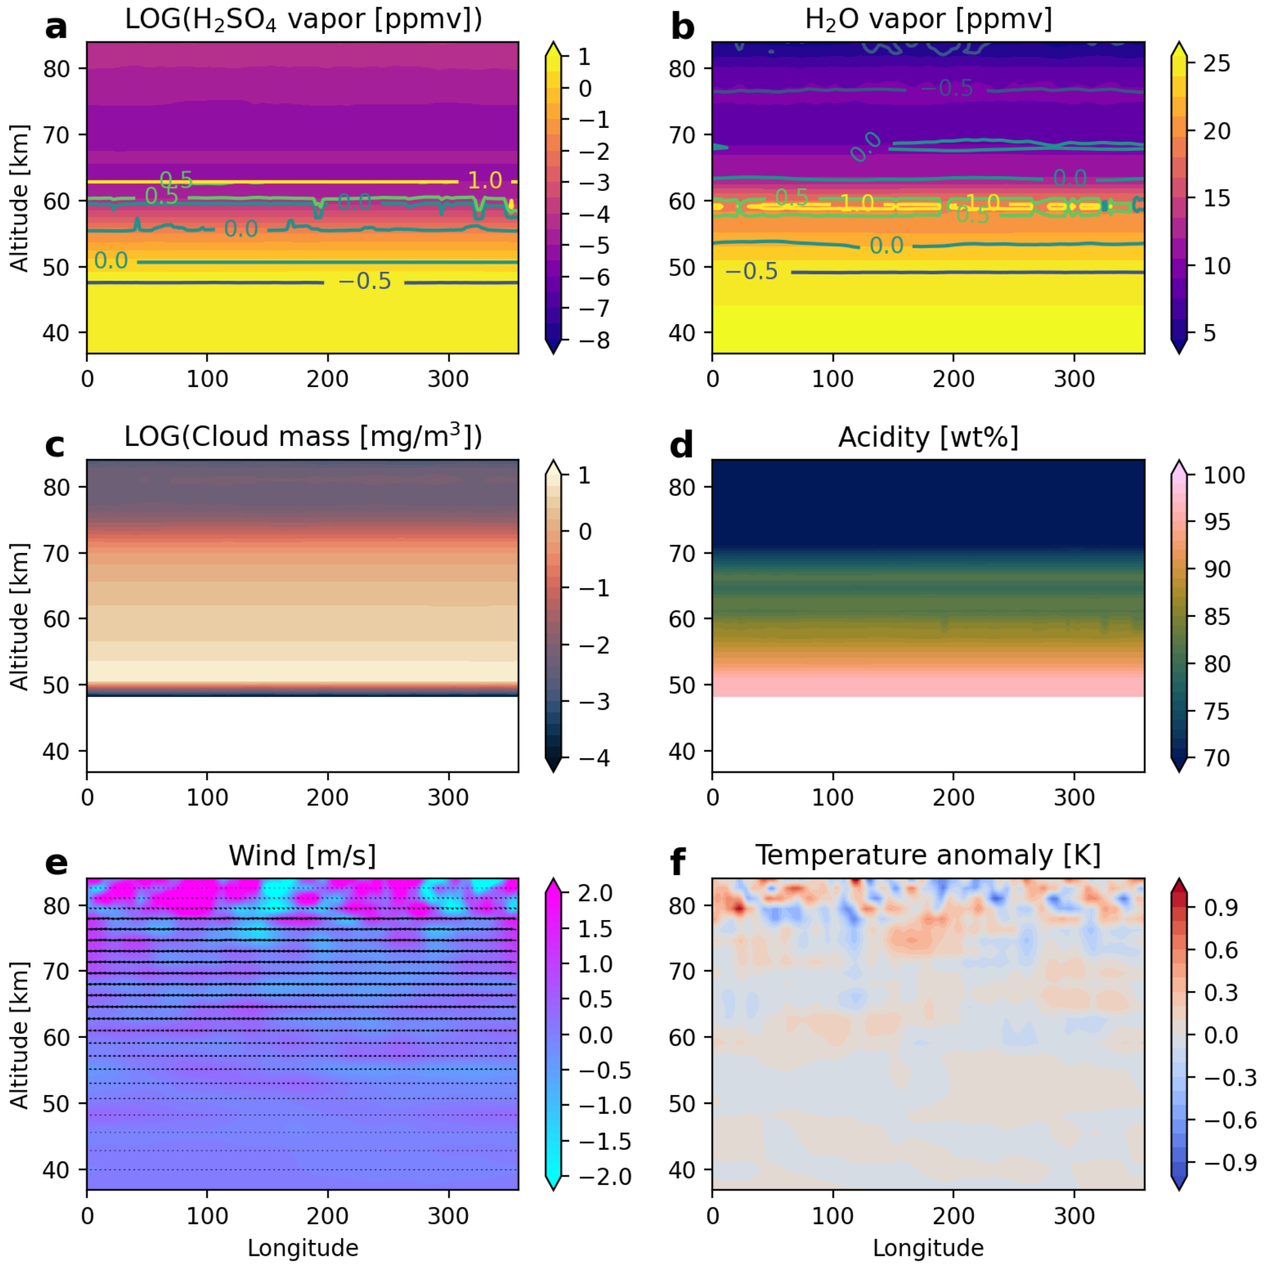


**Figure S2.** Zonal distributions of simulated (a) $H_2SO_4$ vapor (unit: ppmv), (b) $H_2O$ vapor (units: ppmv), (c) cloud mass loading (unit: $mg\,m^{-3}$), (d) cloud acidity (unit: %), (e) wind (unit m/s) and (f) temperature anomaly (unit: K) at the equator averaged over the last Venus solar day. In panel a and b, saturation status is calculated as the relative difference between vapor mixing ration and saturation vapor mixing ratio (SVMR) and shown by solid lines. In panel e, color represents meridional wind; vector indicates zonal and vertical wind, and vertical wind is multiplied by a factor of 1000.

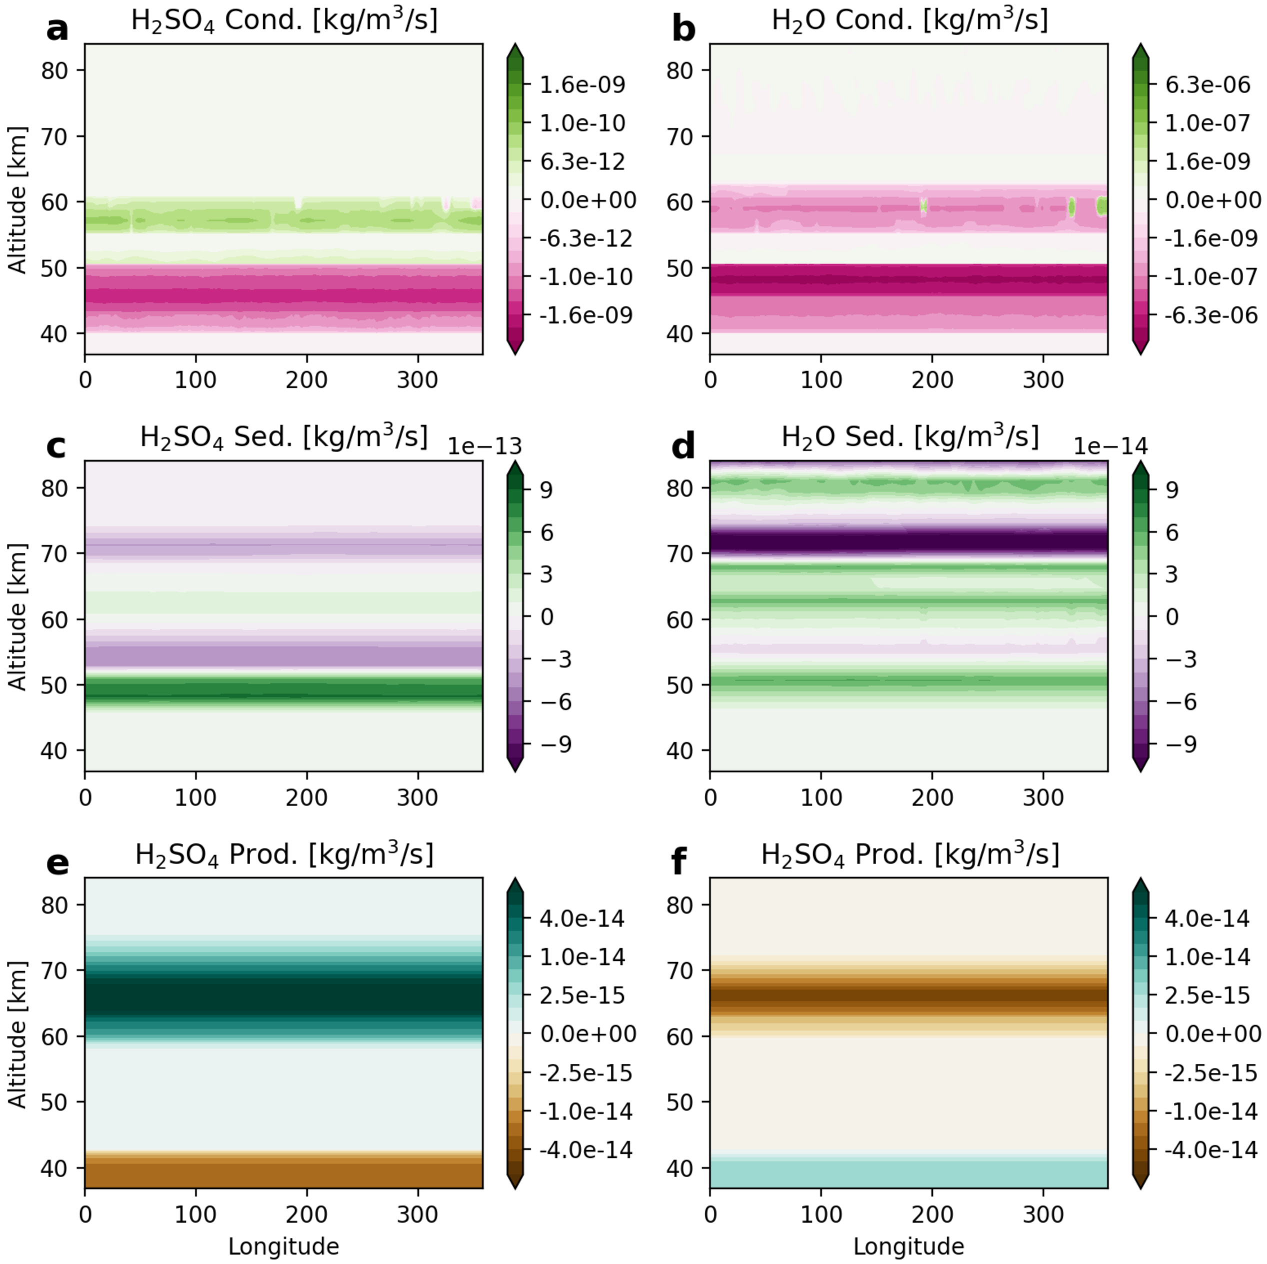


**Figure S3.** Similar to Fig. S1, but for zonal distributions at the equator.

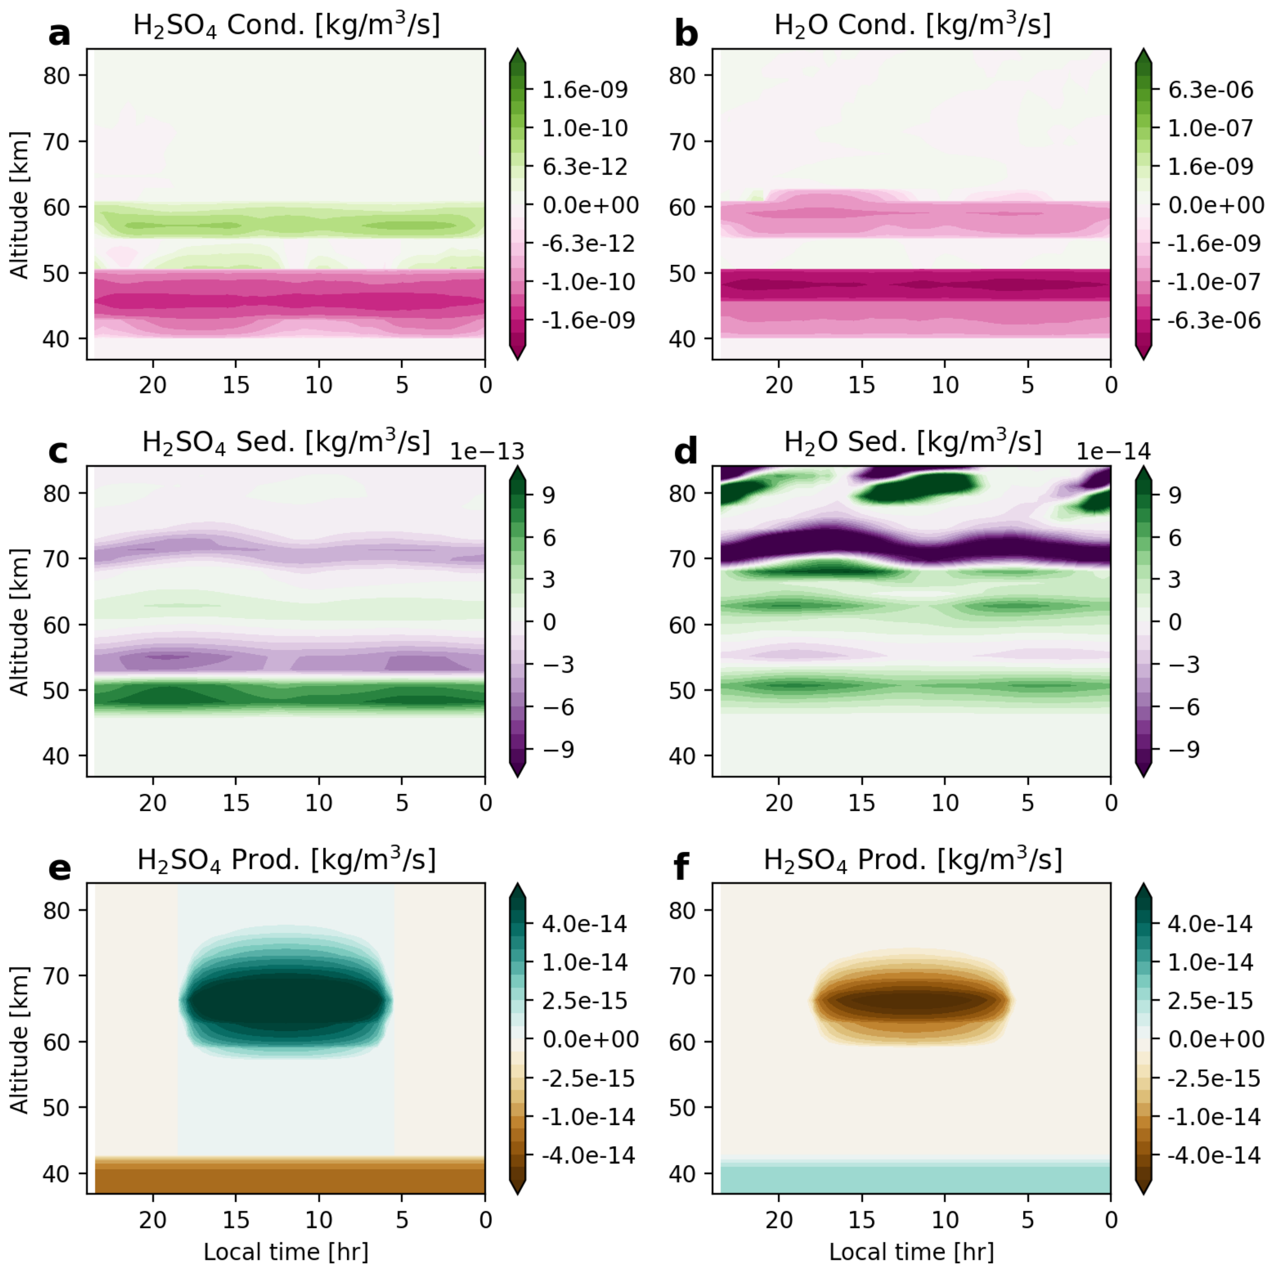


**Figure S4.** Similar to Fig. S1, but for local-time distributions at the equator.

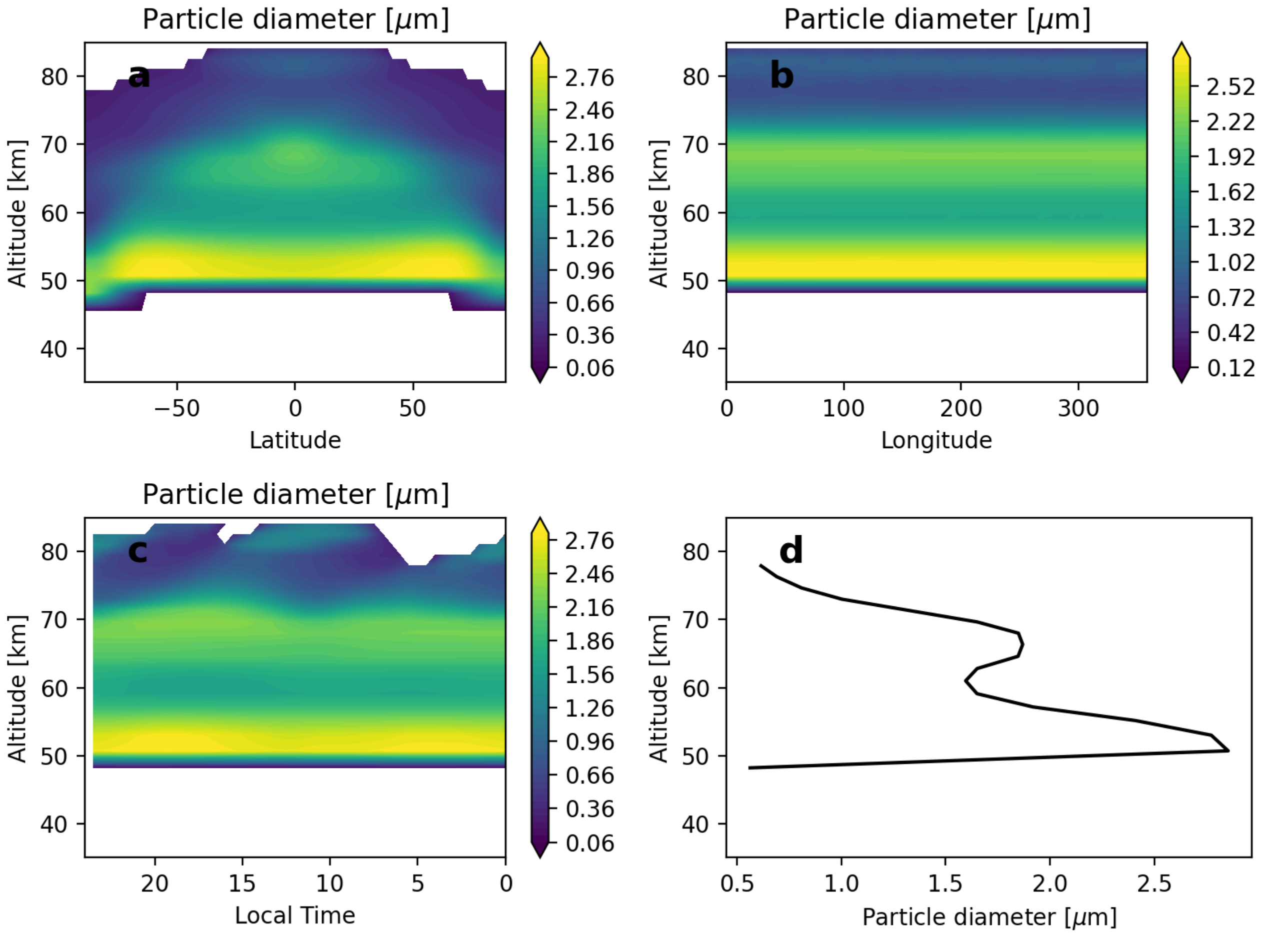


**Figure S5.** Spatial patterns of average cloud particle diameter (unit: $\mu m$) simulated by our model: (a) zonal mean at latitude-altitude plane; (b) zonal distribution at the equator at longitude-altitude plane; (c) local-time distribution at the equator at local-time-altitude plane; (d) global average profile. All the data have been averaged over the last one Venus solar day.

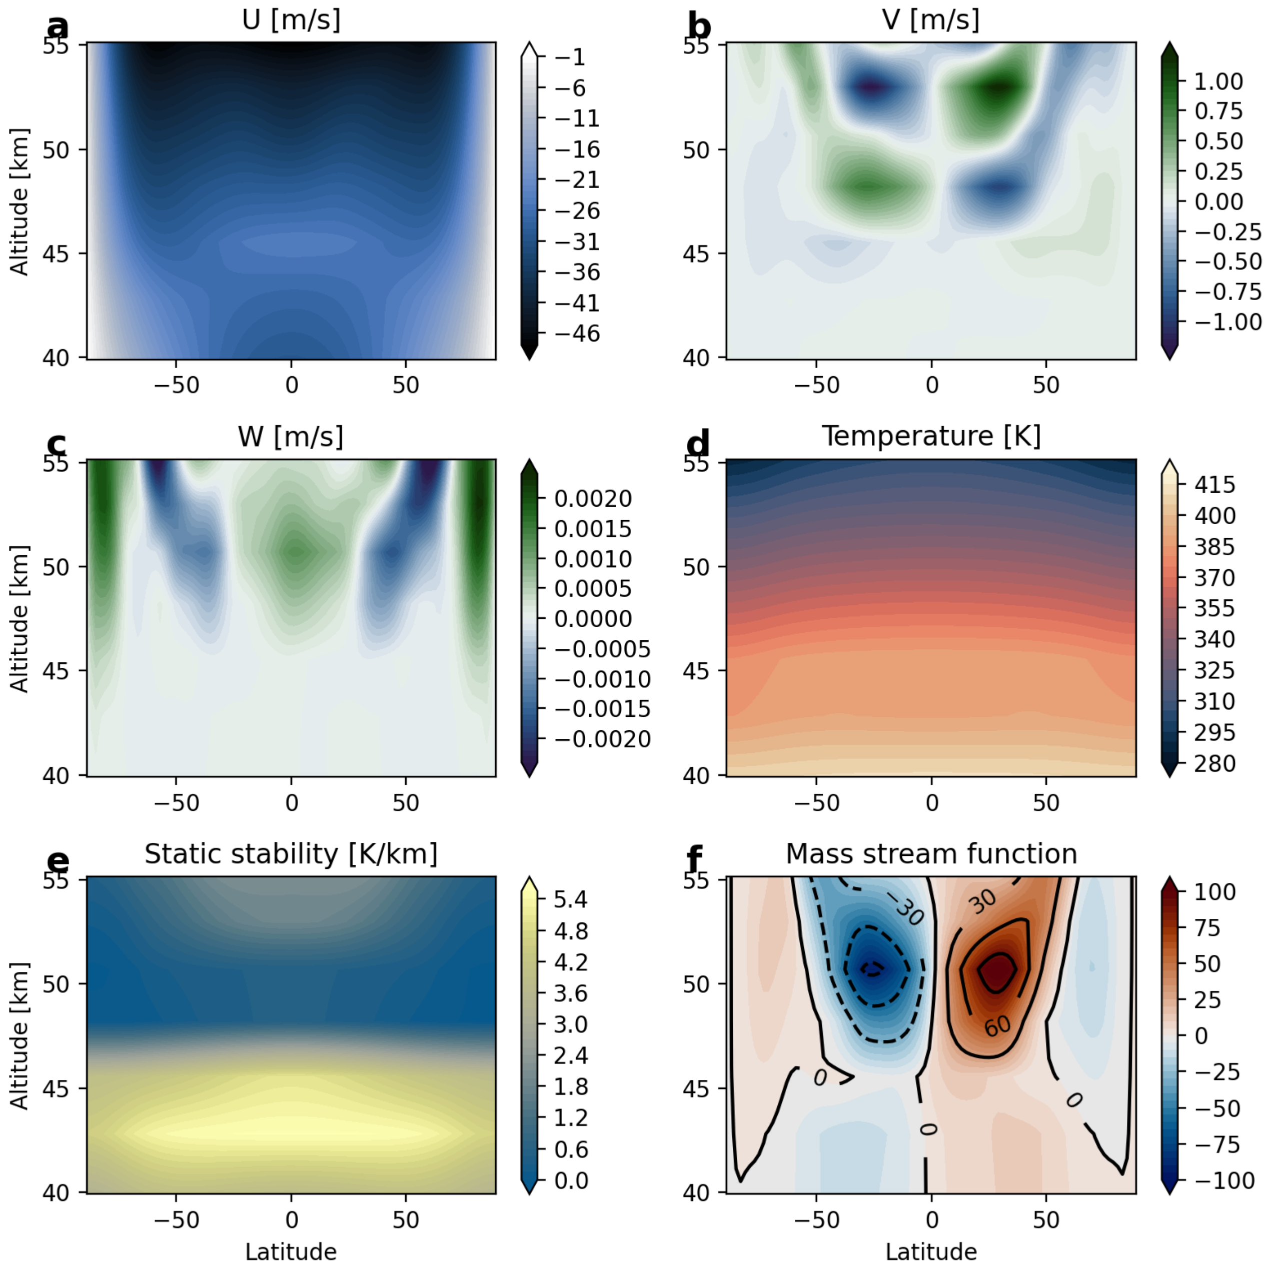


**Figure S6.** Same as Fig.4, but zoomed in for the detailed structure at 40-55 km.

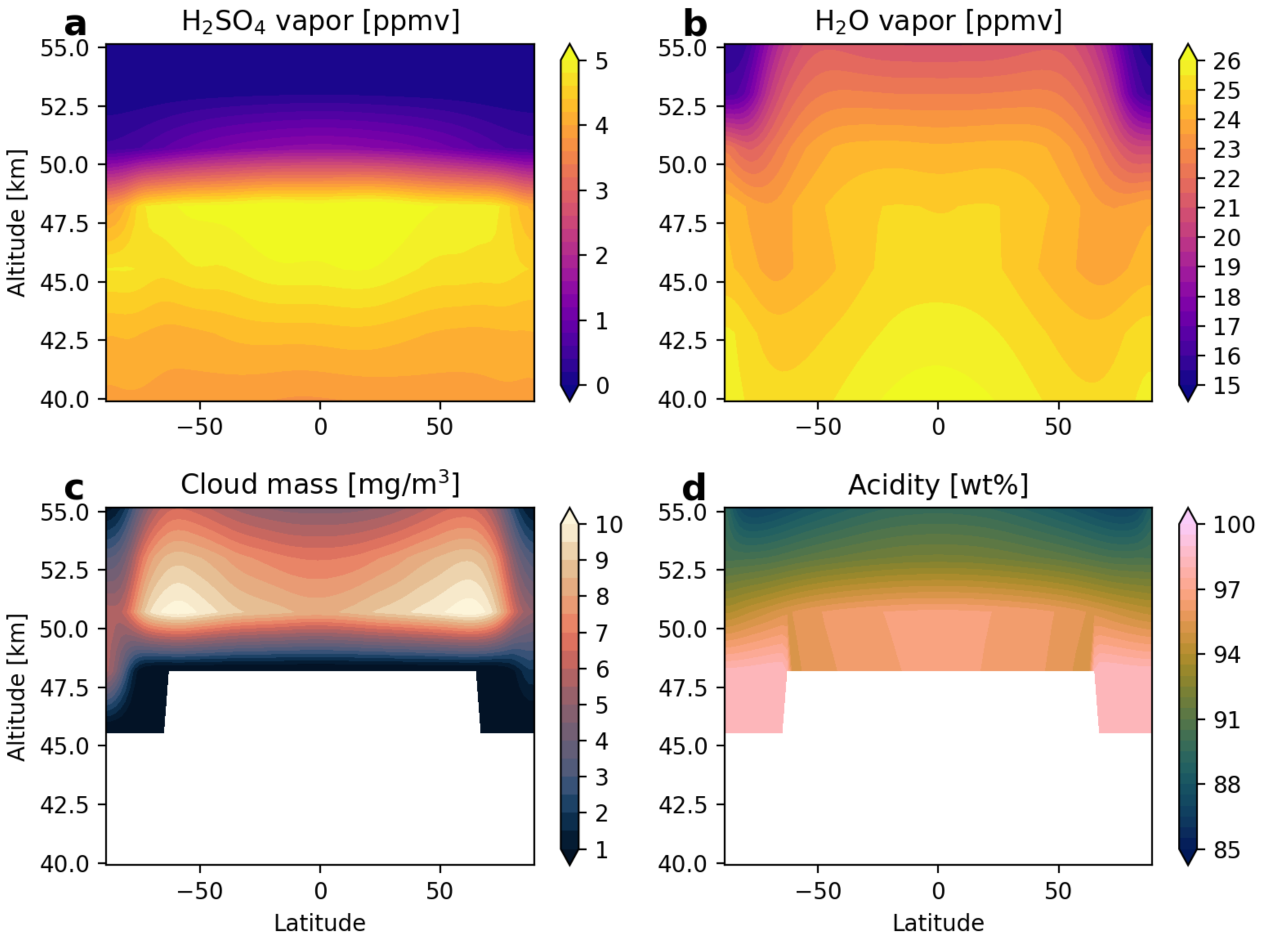


**Figure S7.** Same as Fig.5, but zoomed in for detailed structure at 40-55 km, in order to compare with observations by Oschlisniok et al. (2021).

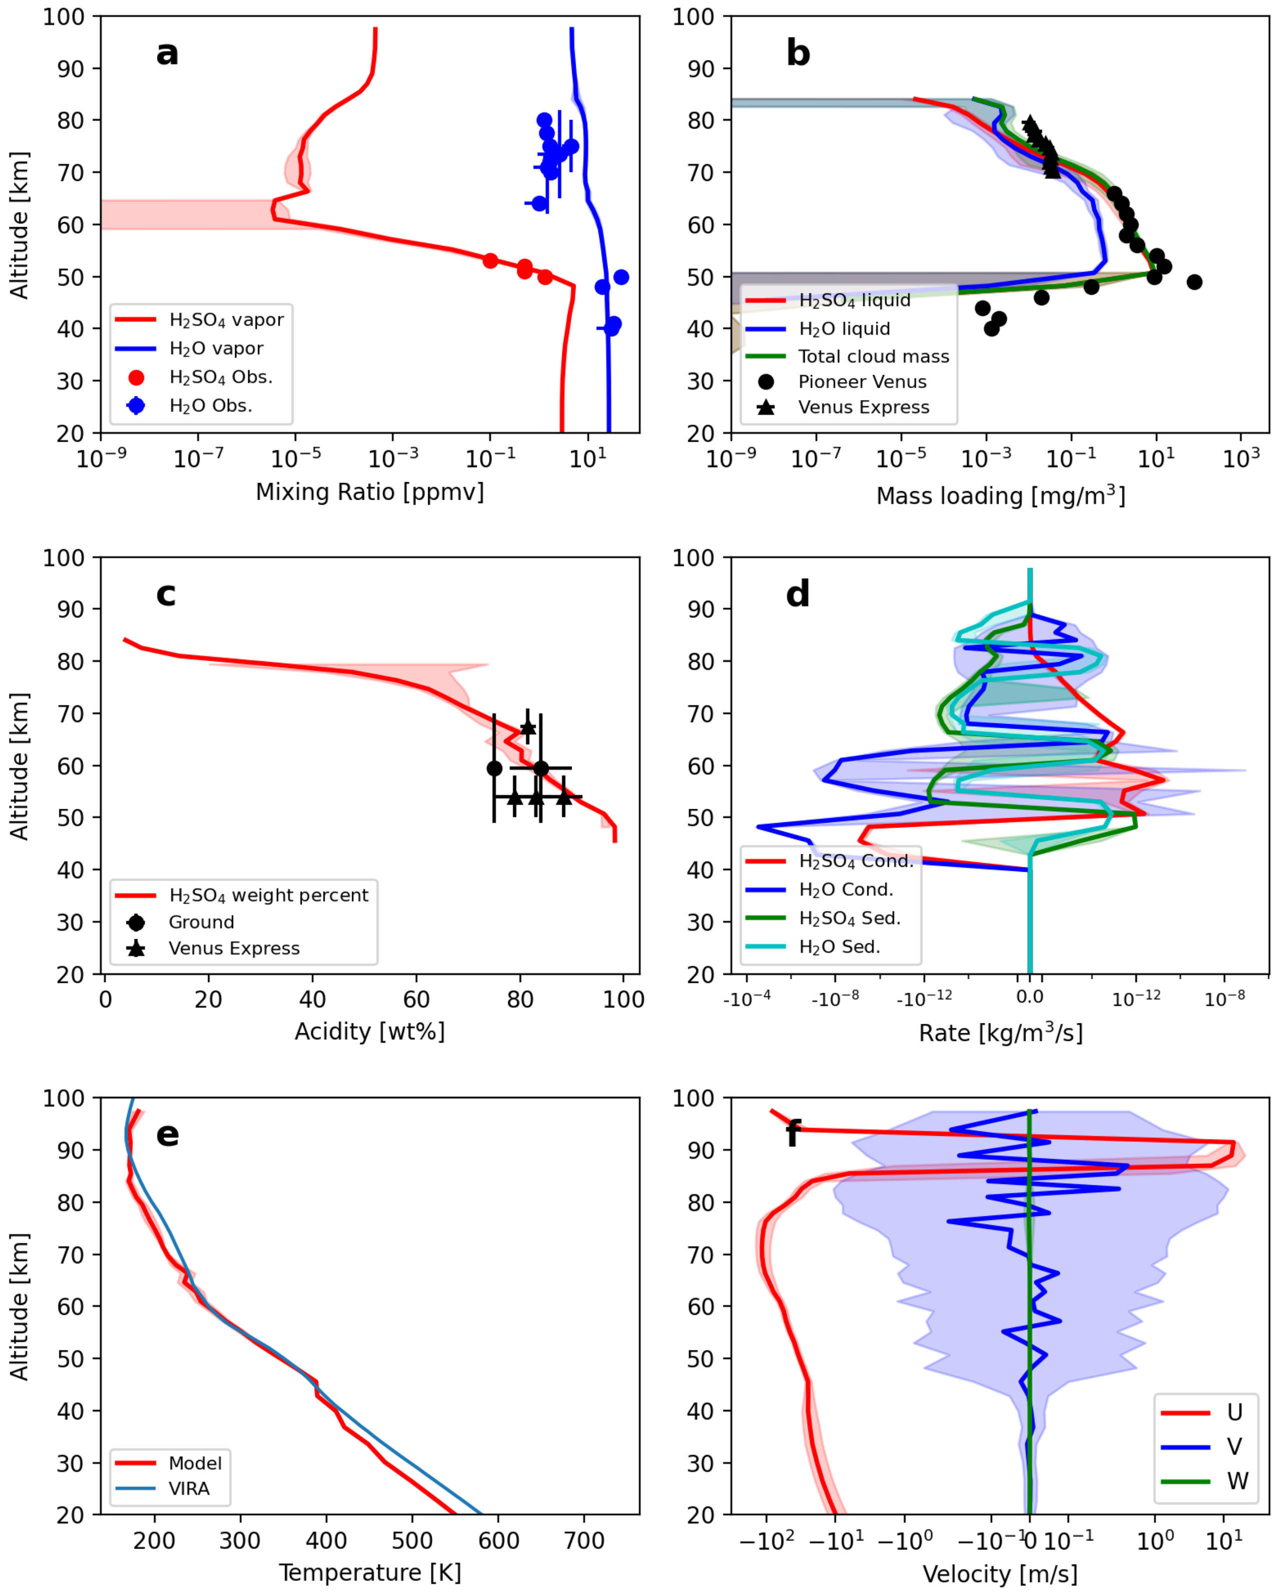


**Figure S8.** Same as Fig.2, but with standard deviations shown by shaded areas.
